# Supplementary material for: The exp-log normal form of types
Source: arXiv:1502.04634 source file (2016-06-30)
Supplement: Supplementary file 1 [file explog-appendix.tex]

\appendix
\section{Formal definitional equalities of the type normalization function}
\begin{coqdoccode}
\coqdockw{Lemma} \coqdocvar{ntimes\_top} : \coqdockw{\ensuremath{\forall}} \coqdocvar{c}, \coqdocvar{ntimes} \coqdocvar{c} \coqdocvar{top} = \coqdocvar{c}.\coqdoceol
\coqdocemptyline
\coqdocindent{0.00em}
\coqdockw{Lemma} \coqdocvar{ntimes\_assoc} :\coqdoceol
\coqdocindent{1.00em}
\coqdockw{\ensuremath{\forall}} \coqdocvar{e1} \coqdocvar{e2} \coqdocvar{e3},\coqdoceol
\coqdocindent{2.00em}
\coqdocvar{ntimes} (\coqdocvar{ntimes} \coqdocvar{e1} \coqdocvar{e2}) \coqdocvar{e3} = \coqdocvar{ntimes} \coqdocvar{e1} (\coqdocvar{ntimes} \coqdocvar{e2} \coqdocvar{e3}).\coqdoceol
\coqdocemptyline
\coqdocindent{0.00em}
\coqdockw{Lemma} \coqdocvar{nplus1\_assoc} :\coqdoceol
\coqdocindent{1.00em}
\coqdockw{\ensuremath{\forall}} \coqdocvar{d} \coqdocvar{e2} \coqdocvar{e3},\coqdoceol
\coqdocindent{2.00em}
\coqdocvar{nplus1} \coqdocvar{d} (\coqdocvar{dnf} (\coqdocvar{nplus} \coqdocvar{e2} \coqdocvar{e3})) = \coqdocvar{nplus1} (\coqdocvar{nplus1} \coqdocvar{d} \coqdocvar{e2}) \coqdocvar{e3}.\coqdoceol
\coqdocemptyline
\coqdocindent{0.00em}
\coqdockw{Lemma} \coqdocvar{nplus\_assoc} :\coqdoceol
\coqdocindent{1.00em}
\coqdockw{\ensuremath{\forall}} \coqdocvar{e1} \coqdocvar{e2} \coqdocvar{e3},\coqdoceol
\coqdocindent{2.00em}
\coqdocvar{nplus} \coqdocvar{e1} (\coqdocvar{dnf} (\coqdocvar{nplus} \coqdocvar{e2} \coqdocvar{e3})) = \coqdocvar{nplus} (\coqdocvar{dnf} (\coqdocvar{nplus} \coqdocvar{e1} \coqdocvar{e2})) \coqdocvar{e3}.\coqdoceol
\coqdocemptyline
\coqdocindent{0.00em}
\coqdockw{Lemma} \coqdocvar{distrib0\_nplus1} :\coqdoceol
\coqdocindent{1.00em}
\coqdockw{\ensuremath{\forall}} \coqdocvar{c} \coqdocvar{d} \coqdocvar{e},\coqdoceol
\coqdocindent{2.00em}
\coqdocvar{distrib0} \coqdocvar{c} (\coqdocvar{nplus1} \coqdocvar{d} \coqdocvar{e}) =\coqdoceol
\coqdocindent{2.00em}
\coqdocvar{dnf} (\coqdocvar{nplus} (\coqdocvar{distrib0} \coqdocvar{c} \coqdocvar{d}) (\coqdocvar{distrib1} \coqdocvar{c} \coqdocvar{e})).\coqdoceol
\coqdocemptyline
\coqdocindent{0.00em}
\coqdockw{Lemma} \coqdocvar{distrib0\_nplus} :\coqdoceol
\coqdocindent{1.00em}
\coqdockw{\ensuremath{\forall}} \coqdocvar{c} \coqdocvar{e1} \coqdocvar{e2},\coqdoceol
\coqdocindent{2.00em}
\coqdocvar{distrib0} \coqdocvar{c} (\coqdocvar{nplus} \coqdocvar{e1} \coqdocvar{e2}) =\coqdoceol
\coqdocindent{2.00em}
\coqdocvar{dnf} (\coqdocvar{nplus} (\coqdocvar{distrib1} \coqdocvar{c} \coqdocvar{e1}) (\coqdocvar{distrib1} \coqdocvar{c} \coqdocvar{e2})).\coqdoceol
\coqdocemptyline
\coqdocindent{0.00em}
\coqdockw{Lemma} \coqdocvar{distribn\_nplus1} :\coqdoceol
\coqdocindent{1.00em}
\coqdockw{\ensuremath{\forall}} \coqdocvar{d} \coqdocvar{e1} \coqdocvar{e2},\coqdoceol
\coqdocindent{2.00em}
\coqdocvar{distribn} (\coqdocvar{nplus1} \coqdocvar{d} \coqdocvar{e1}) \coqdocvar{e2} =\coqdoceol
\coqdocindent{2.00em}
\coqdocvar{dnf} (\coqdocvar{nplus} (\coqdocvar{distribn} \coqdocvar{d} \coqdocvar{e2}) (\coqdocvar{distrib} \coqdocvar{e1} \coqdocvar{e2})).\coqdoceol
\coqdocemptyline
\coqdocindent{0.00em}
\coqdockw{Lemma} \coqdocvar{distribn\_nplus} :\coqdoceol
\coqdocindent{1.00em}
\coqdockw{\ensuremath{\forall}} \coqdocvar{e1} \coqdocvar{e2} \coqdocvar{e3},\coqdoceol
\coqdocindent{2.00em}
\coqdocvar{distribn} (\coqdocvar{nplus} \coqdocvar{e1} \coqdocvar{e2}) \coqdocvar{e3} =\coqdoceol
\coqdocindent{2.00em}
\coqdocvar{dnf} (\coqdocvar{nplus} (\coqdocvar{distrib} \coqdocvar{e1} \coqdocvar{e3}) (\coqdocvar{distrib} \coqdocvar{e2} \coqdocvar{e3})).\coqdoceol
\coqdocemptyline
\coqdocindent{0.00em}
\coqdockw{Lemma} \coqdocvar{distrib1\_top} : \coqdockw{\ensuremath{\forall}} \coqdocvar{e}, \coqdocvar{distrib1} \coqdocvar{top} \coqdocvar{e} = \coqdocvar{e}.\coqdoceol
\coqdocemptyline
\coqdocindent{0.00em}
\coqdockw{Lemma} \coqdocvar{distrib1\_distrib0} :\coqdoceol
\coqdocindent{1.00em}
\coqdockw{\ensuremath{\forall}} \coqdocvar{c} \coqdocvar{c0} \coqdocvar{d},\coqdoceol
\coqdocindent{2.00em}
\coqdocvar{distrib1} \coqdocvar{c} (\coqdocvar{distrib0} \coqdocvar{c0} \coqdocvar{d}) = \coqdocvar{distrib0} (\coqdocvar{ntimes} \coqdocvar{c} \coqdocvar{c0}) \coqdocvar{d}.\coqdoceol
\coqdocemptyline
\coqdocindent{0.00em}
\coqdockw{Lemma} \coqdocvar{distrib1\_distrib1} :\coqdoceol
\coqdocindent{1.00em}
\coqdockw{\ensuremath{\forall}} \coqdocvar{c} \coqdocvar{c0} \coqdocvar{e3}, \coqdoceol
\coqdocindent{2.00em}
\coqdocvar{distrib1} \coqdocvar{c} (\coqdocvar{distrib1} \coqdocvar{c0} \coqdocvar{e3}) = \coqdocvar{distrib1} (\coqdocvar{ntimes} \coqdocvar{c} \coqdocvar{c0}) \coqdocvar{e3}.\coqdoceol
\coqdocemptyline
\coqdocindent{0.00em}
\coqdockw{Lemma} \coqdocvar{distrib1\_distribn} :\coqdoceol
\coqdocindent{1.00em}
\coqdockw{\ensuremath{\forall}} \coqdocvar{c} \coqdocvar{d} \coqdocvar{e3},\coqdoceol
\coqdocindent{2.00em}
\coqdocvar{distrib1} \coqdocvar{c} (\coqdocvar{distribn} \coqdocvar{d} \coqdocvar{e3}) = \coqdocvar{distrib} (\coqdocvar{distrib0} \coqdocvar{c} \coqdocvar{d}) \coqdocvar{e3}.\coqdoceol
\coqdocemptyline
\coqdocindent{0.00em}
\coqdockw{Lemma} \coqdocvar{distrib1\_distrib} :\coqdoceol
\coqdocindent{1.00em}
\coqdockw{\ensuremath{\forall}} \coqdocvar{c} \coqdocvar{e2} \coqdocvar{e3},\coqdoceol
\coqdocindent{2.00em}
\coqdocvar{distrib1} \coqdocvar{c} (\coqdocvar{distrib} \coqdocvar{e2} \coqdocvar{e3}) = \coqdocvar{distrib} (\coqdocvar{distrib1} \coqdocvar{c} \coqdocvar{e2}) \coqdocvar{e3}.\coqdoceol
\coqdocemptyline
\coqdocindent{0.00em}
\coqdockw{Lemma} \coqdocvar{distribn\_distrib} :\coqdoceol
\coqdocindent{1.00em}
\coqdockw{\ensuremath{\forall}} \coqdocvar{d} \coqdocvar{e2} \coqdocvar{e3},\coqdoceol
\coqdocindent{2.00em}
\coqdocvar{distribn} \coqdocvar{d} (\coqdocvar{distrib} \coqdocvar{e2} \coqdocvar{e3}) = \coqdocvar{distrib} (\coqdocvar{distribn} \coqdocvar{d} \coqdocvar{e2}) \coqdocvar{e3}.\coqdoceol
\coqdocemptyline
\coqdocindent{0.00em}
\coqdockw{Lemma} \coqdocvar{distrib\_assoc} :\coqdoceol
\coqdocindent{1.00em}
\coqdockw{\ensuremath{\forall}} \coqdocvar{e1} \coqdocvar{e2} \coqdocvar{e3},\coqdoceol
\coqdocindent{2.00em}
\coqdocvar{distrib} \coqdocvar{e1} (\coqdocvar{distrib} \coqdocvar{e2} \coqdocvar{e3}) = \coqdocvar{distrib} (\coqdocvar{distrib} \coqdocvar{e1} \coqdocvar{e2}) \coqdocvar{e3}.\coqdoceol
\coqdocemptyline
\coqdocindent{0.00em}
\coqdockw{Lemma} \coqdocvar{explogn\_top} : \coqdockw{\ensuremath{\forall}} \coqdocvar{c}, \coqdocvar{explogn} \coqdocvar{c} (\coqdocvar{cnf} \coqdocvar{top}) = \coqdocvar{c}.\coqdoceol
\coqdocemptyline
\coqdocindent{0.00em}
\coqdockw{Lemma} \coqdocvar{explogn\_ntimes} :\coqdoceol
\coqdocindent{1.00em}
\coqdockw{\ensuremath{\forall}} \coqdocvar{c} \coqdocvar{c'} \coqdocvar{e},\coqdoceol
\coqdocindent{2.00em}
\coqdocvar{explogn} (\coqdocvar{ntimes} \coqdocvar{c} \coqdocvar{c'}) \coqdocvar{e} =\coqdoceol
\coqdocindent{2.00em}
\coqdocvar{ntimes} (\coqdocvar{explogn} \coqdocvar{c} \coqdocvar{e}) (\coqdocvar{explogn} \coqdocvar{c'} \coqdocvar{e}).\coqdoceol
\coqdocemptyline
\coqdocindent{0.00em}
\coqdockw{Lemma} \coqdocvar{explog0\_nplus1} :\coqdoceol
\coqdocindent{1.00em}
\coqdockw{\ensuremath{\forall}} \coqdocvar{b} \coqdocvar{d} \coqdocvar{e},\coqdoceol
\coqdocindent{2.00em}
\coqdocvar{explog0} \coqdocvar{b} (\coqdocvar{nplus1} \coqdocvar{d} \coqdocvar{e}) = \coqdocvar{ntimes} (\coqdocvar{explog0} \coqdocvar{b} \coqdocvar{d}) (\coqdocvar{explog1} \coqdocvar{b} \coqdocvar{e}).\coqdoceol
\coqdocemptyline
\coqdocindent{0.00em}
\coqdockw{Lemma} \coqdocvar{explog0\_nplus} :\coqdoceol
\coqdocindent{1.00em}
\coqdockw{\ensuremath{\forall}} \coqdocvar{b} \coqdocvar{e1} \coqdocvar{e2},\coqdoceol
\coqdocindent{2.00em}
\coqdocvar{explog0} \coqdocvar{b} (\coqdocvar{nplus} \coqdocvar{e1} \coqdocvar{e2}) = \coqdocvar{ntimes} (\coqdocvar{explog1} \coqdocvar{b} \coqdocvar{e1}) (\coqdocvar{explog1} \coqdocvar{b} \coqdocvar{e2}).\coqdoceol
\coqdocemptyline
\coqdocindent{0.00em}
\coqdockw{Lemma} \coqdocvar{explogn\_explog1} :\coqdoceol
\coqdocindent{1.00em}
\coqdockw{\ensuremath{\forall}} \coqdocvar{b} \coqdocvar{e1} \coqdocvar{e2},\coqdoceol
\coqdocindent{2.00em}
\coqdocvar{explogn} (\coqdocvar{explog1} \coqdocvar{b} \coqdocvar{e1}) \coqdocvar{e2} = \coqdocvar{explog1} \coqdocvar{b} (\coqdocvar{distrib} \coqdocvar{e1} \coqdocvar{e2}).\coqdoceol
\coqdocemptyline
\coqdocindent{0.00em}
\coqdockw{Lemma} \coqdocvar{explogn\_distrib} : \coqdockw{\ensuremath{\forall}} \coqdocvar{c} \coqdocvar{e1} \coqdocvar{e2},\coqdoceol
\coqdocindent{2.00em}
\coqdocvar{explogn} \coqdocvar{c} (\coqdocvar{distrib} \coqdocvar{e1} \coqdocvar{e2}) = \coqdocvar{explogn} (\coqdocvar{explogn} \coqdocvar{c} \coqdocvar{e1}) \coqdocvar{e2}.\coqdoceol
\end{coqdoccode}
%%% Local Variables:
%%% mode: latex
%%% TeX-master: "explog"
%%% End:
